# Supplementary material for: Nonlinear thermoplasmonics in graphene nanostructures
Source: arXiv:2408.14798 source file (2024-08-27)
Supplement: Supplementary file 1 [file supplement.tex]

\documentclass[superscriptaddress,nofootinbib,amsmath,amssymb,aps,pra,onecolumn]{revtex4-2}

\usepackage{amsmath}
\usepackage{amssymb}
\usepackage{amsfonts}
\usepackage{bm} % bold math
\usepackage{bbm}
\usepackage{braket}
\usepackage{color}
\usepackage{comment}
\usepackage{dcolumn} % align table columns on decimal point
\usepackage{dsfont}
\usepackage{enumerate}
\usepackage{epsfig}
\usepackage{esint}
\usepackage[T1]{fontenc}
\usepackage{framed}
\usepackage{gensymb}
\usepackage{graphicx} % include figure files
\usepackage[colorlinks,linkcolor=blue,citecolor=blue,urlcolor=blue,hyperindex,driverfallback=dvipdfm]{hyperref}
\usepackage{indentfirst}
\usepackage{lmodern}
\usepackage{mathrsfs}
\usepackage{mathtools}
\usepackage{multirow}
\usepackage{psfrag}
\usepackage{pst-all}
\usepackage{soul}
\usepackage{xcolor}
\usepackage{xspace}
\usepackage{orcidlink}

% --- parentheses ---

% --- math/physical constants/symbols ---

% --- spatial and momentum coordinates, etc. ---

% --- EM fields, dipoles, etc. ---
  
% --- common physics definitions ---
    % solid-state, Fermi energy, etc.
% --- misc. re-definitions ---
  
% --- frequency domain definitions ---
\def\ww{\omega}
% --- calligraphic definitions ---
  
% --- misc. electromagnetic definitions ---
    % induced and external scalar potential

\mathtoolsset{showonlyrefs} % label only referred equations

\begin{document}

\title{Nonlinear thermoplasmonics in graphene nanostructures \\ {\color{gray} \small -- SUPPORTING INFORMATION --}}

\author{Line Jelver\,\orcidlink{0000-0001-5503-5604}}
\affiliation{POLIMA---Center for Polariton-driven Light--Matter Interactions, University of Southern Denmark, Campusvej 55, DK-5230 Odense M, Denmark}

\author{Joel~D.~Cox\,\orcidlink{0000-0002-5954-6038}}
\email[Joel~D.~Cox: ]{cox@mci.sdu.dk}
\affiliation{POLIMA---Center for Polariton-driven Light--Matter Interactions, University of Southern Denmark, Campusvej 55, DK-5230 Odense M, Denmark}
\affiliation{Danish Institute for Advanced Study, University of Southern Denmark, Campusvej 55, DK-5230 Odense M, Denmark}

\begin{abstract}
We compare the linear optical response of narrow graphene nanoribbons (GNRs) predicted in the random phase approximation using Wannier tight-binding models with corresponding results obtained from direct ab-initio calculations, present additional simulations of the electronic distribution and optical response as functions of added thermal energy in GNRs of varying width, and show additional results exploring the evolution of plasmons in GNRs with both electron and hole doping.
\end{abstract}

\date{\today}
\maketitle
%\tableofcontents

%%%%%%%%%%%%%%%%%%%%%%%%%%%%%%%%%%%%%%%%%%%%%%%%%%%%%%%%%%%%%%%%%%%%%%%%%%%%%%%

\begin{figure*}
    \centering
    \includegraphics[width=0.8\textwidth]{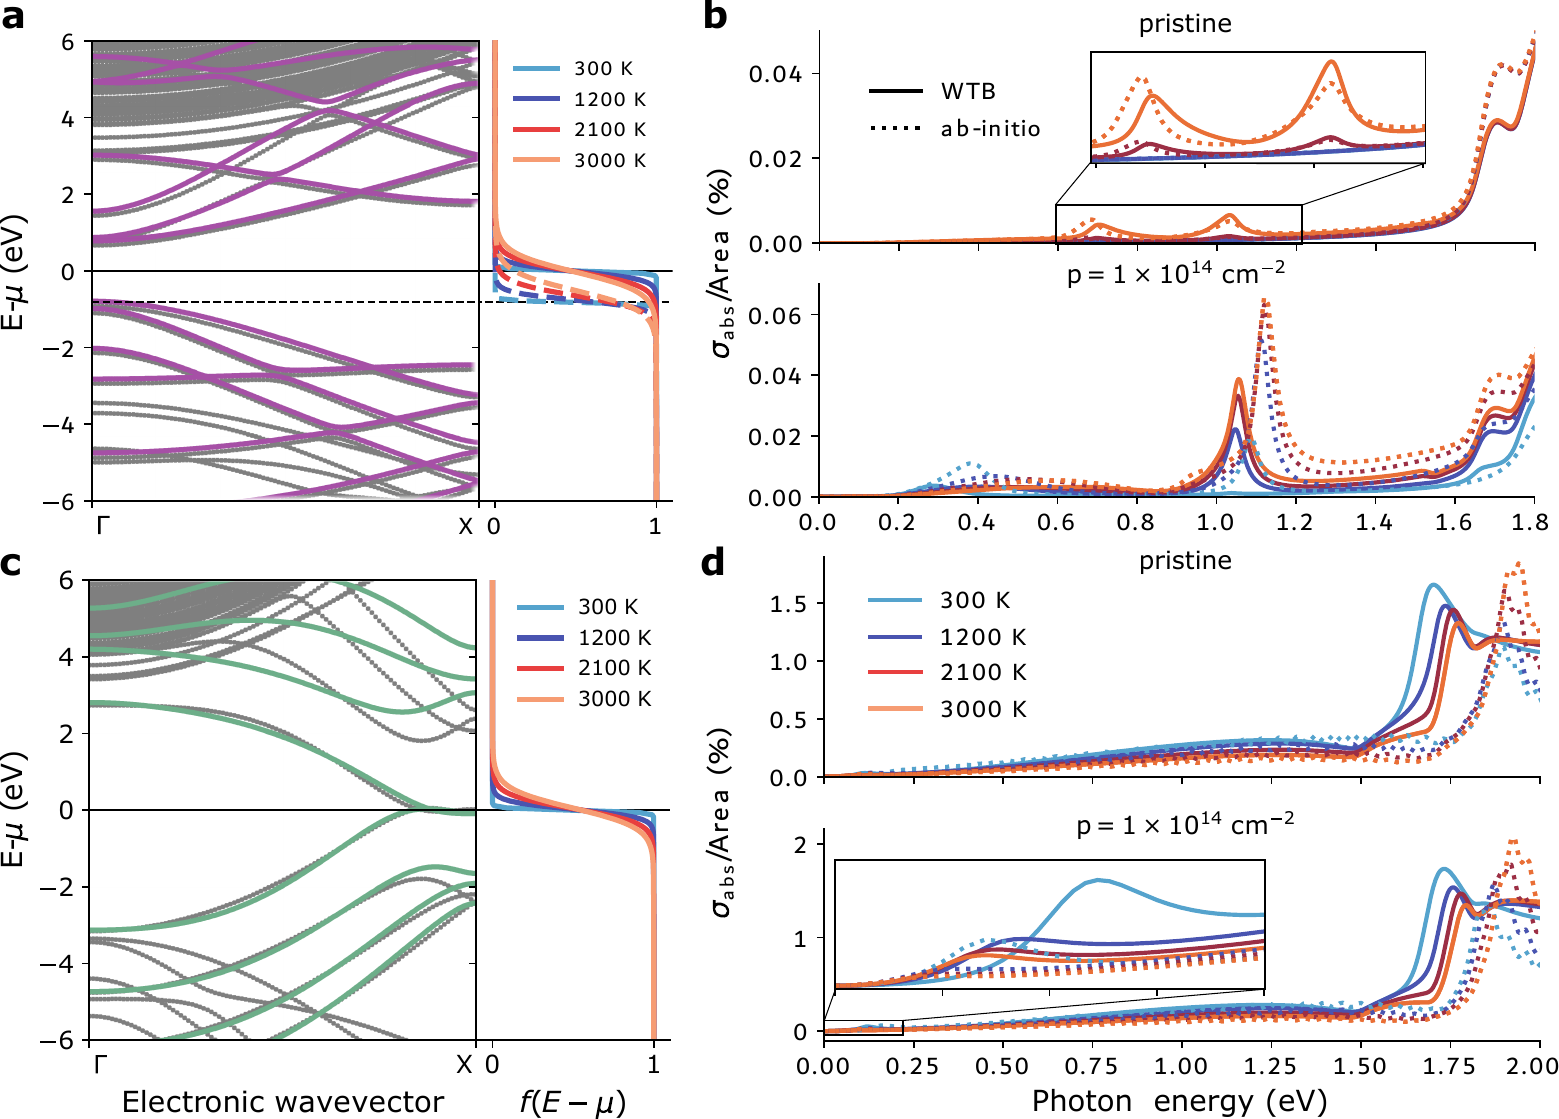}
    \caption{\textbf{Comparison of electronic states and optical response in Wannier tight-binding and direct ab-initio calculations.} The electronic bands of narrow GNRs with \textbf{a} armchair (7-aGNR) and \textbf{b} zigzag (8-zGNR) edge terminations computed using the Wannier tight-binding (WTB) approach described in the main text (based on the Quantum Espresso code, colored curves) are compared with ab-initio bands computed using the Yambo code (grey curves) \cite{marini2009yambo,sangalli2019manybody}, together with the occupation functions at the indicated temperatures (right panels). In right panel of \textbf{a}, the Fermi level (dotted horizontal line) and occupation functions for a hole doping density $p=10^{14}$\,cm$^{-2}$ (dashed curves) are shown, while in the 8-zGNR these quantities are almost unchanged between the pristine case and the considered doping level due to the filling of edge states. The corresponding linear absorption cross section of the \textbf{c} 7-aGNR and \textbf{d} 8-zGNR obtained using the WTB (solid curves) and ab-initio (dotted curves) models are presented for both pristine (upper panels) and hole-doped (lower panels) ribbons. Ab-initio calculations include the 20 closest electronic bands around the Fermi level, sampling 201 and 501 k-points in the periodic direction for the armchair and zigzag edge-terminated ribbon, respectively. Note that the wiggles in the ab-initio results appearing at higher energies are an artefact of insufficient k-point sampling.}
    \label{fig:figS1}
\end{figure*}

\begin{figure*}
    \centering
    \includegraphics[width=0.99\textwidth]{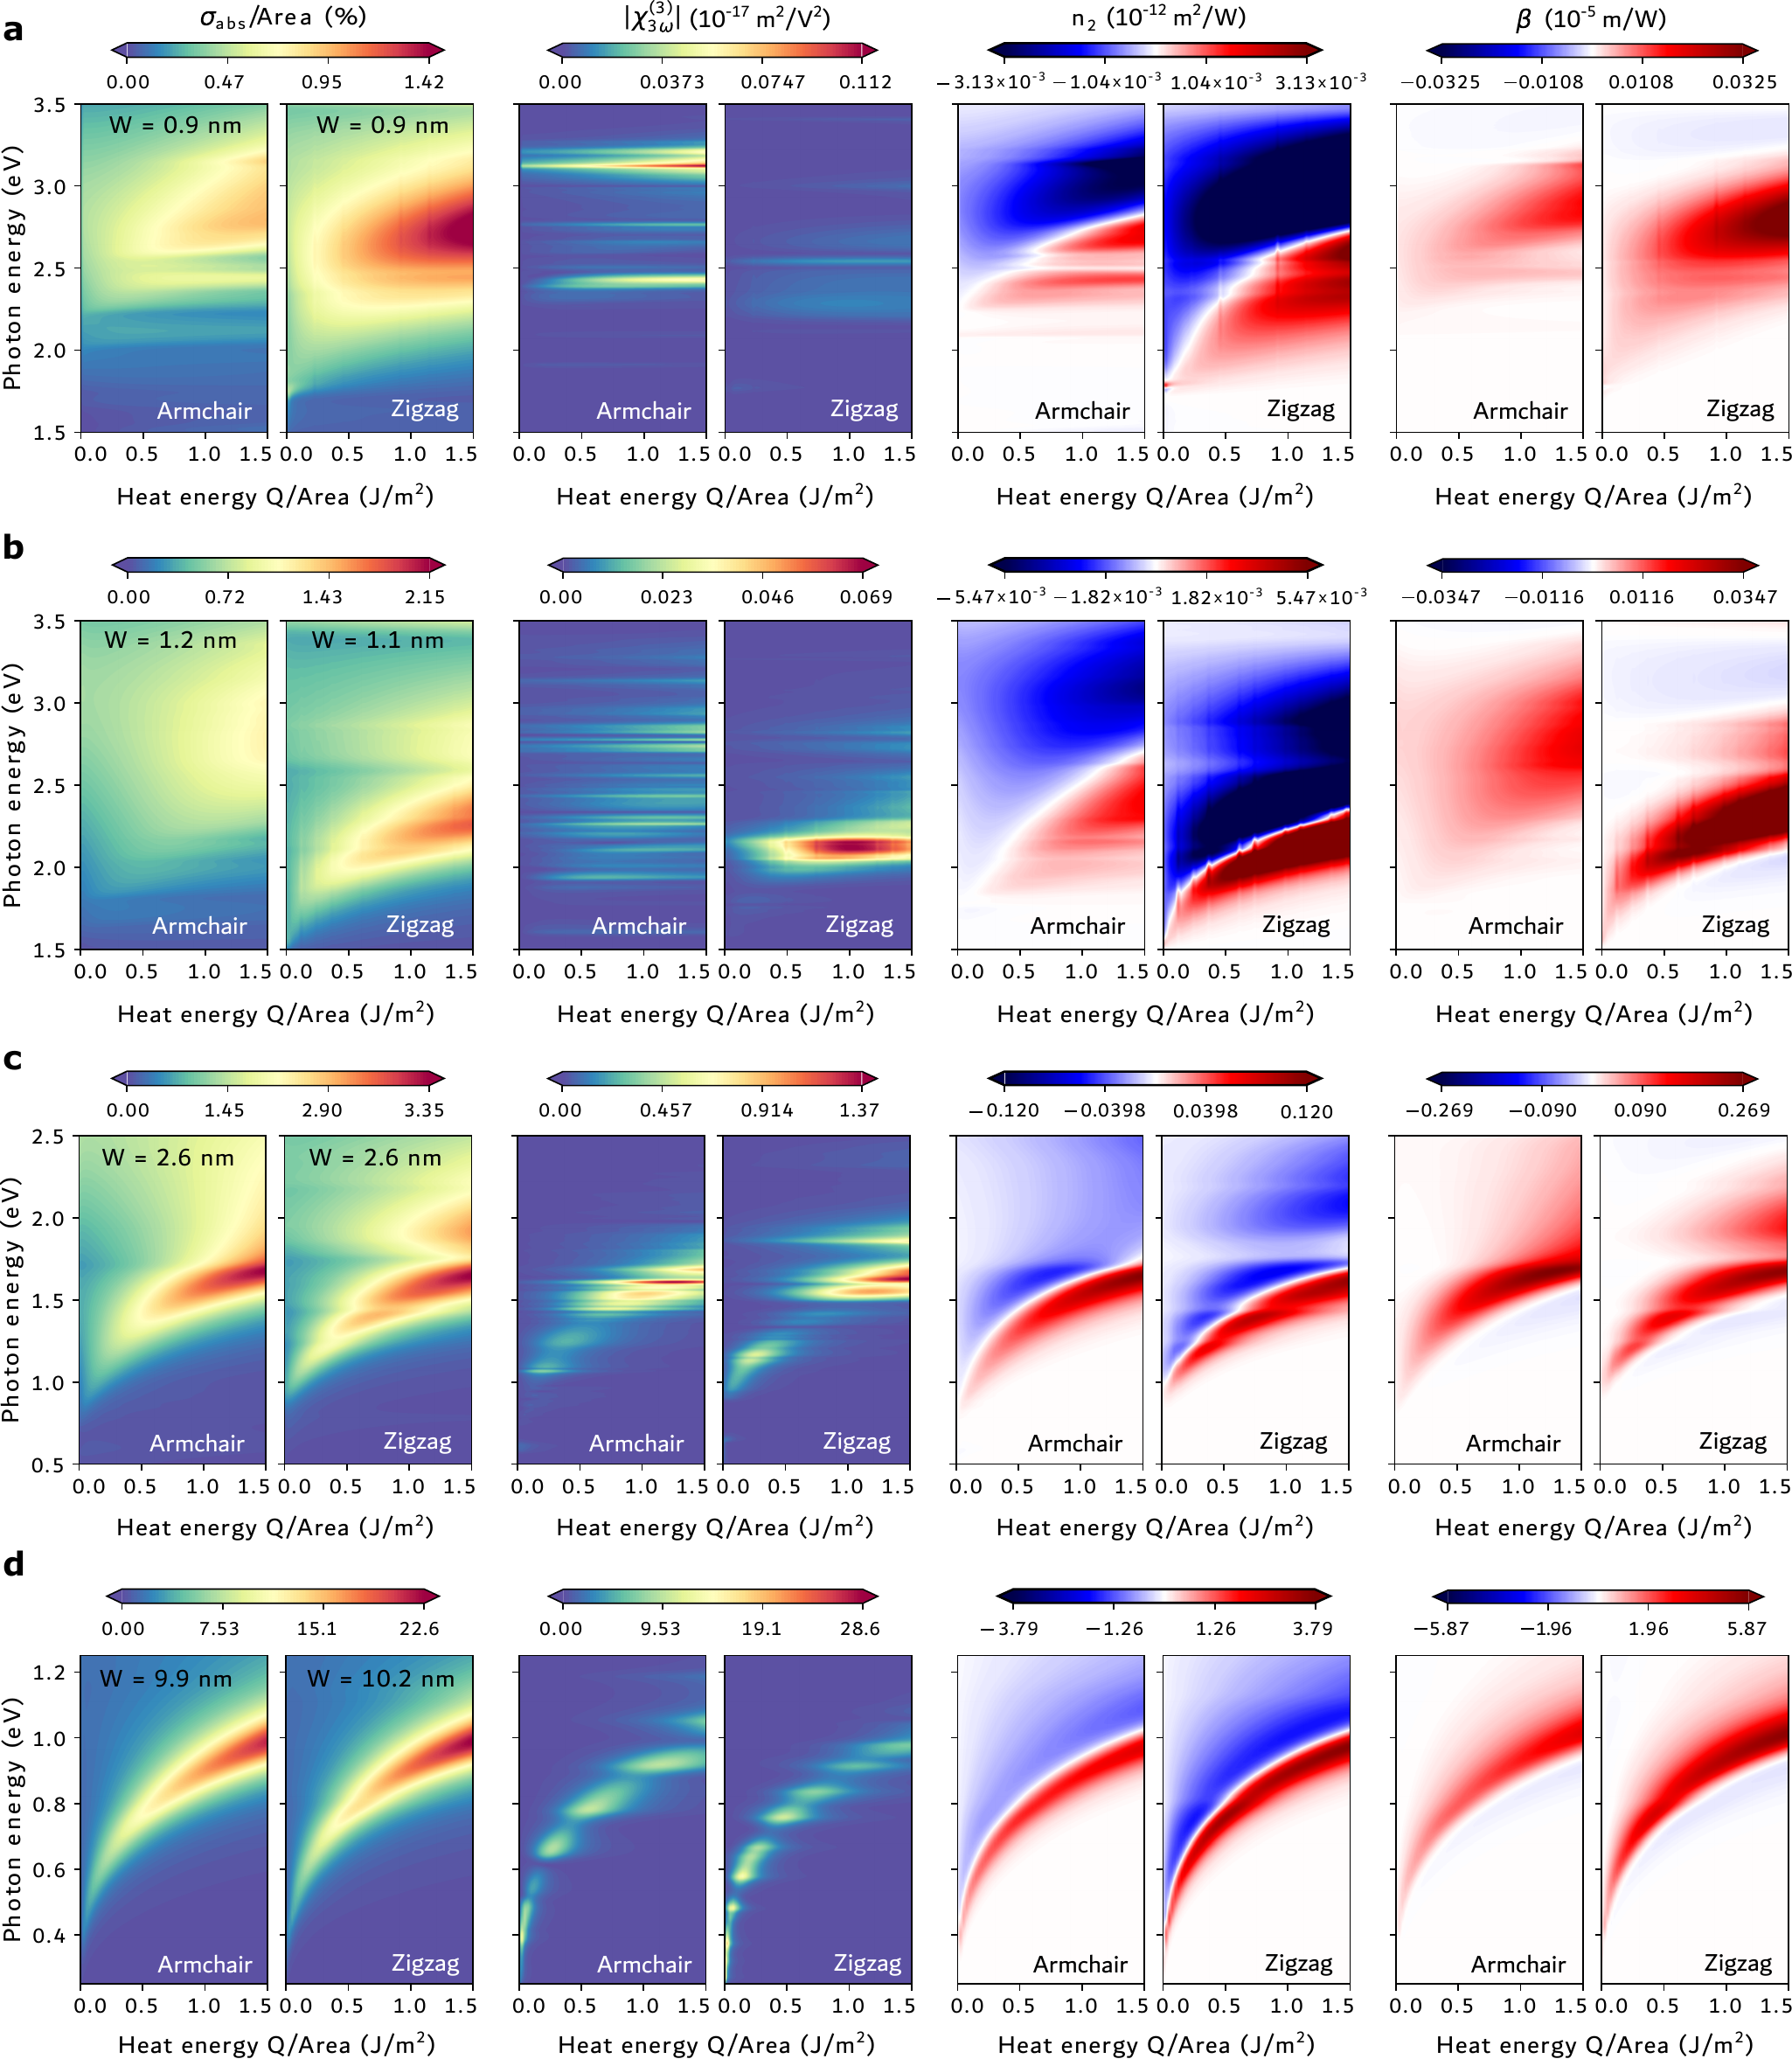}
    \caption{\textbf{Tunability of thermoplasmons in graphene nanoribbons of varying width.} The linear absorption cross section $\sigma^{\rm abs}$, third-harmonic susceptibility $\chi_{3\ww}^{(3)}$, nonlinear refractive index $n_2$, and two-photon absorption coefficient $\beta$ calculated for armchair and zigzag GNRs of widths \textbf{a} $W\approx 0.9$\,nm, \textbf{b} $W\approx1.1$\,nm, \textbf{c} $W\approx 2.6$\,nm, and \textbf{d} $W\approx 10$\,nm are shown as functions of the added heat energy $Q$ per unit area and the photon energy.}
    \label{fig:figS2}
\end{figure*}

\begin{figure*}
    \centering
    \includegraphics[width=0.9\textwidth]{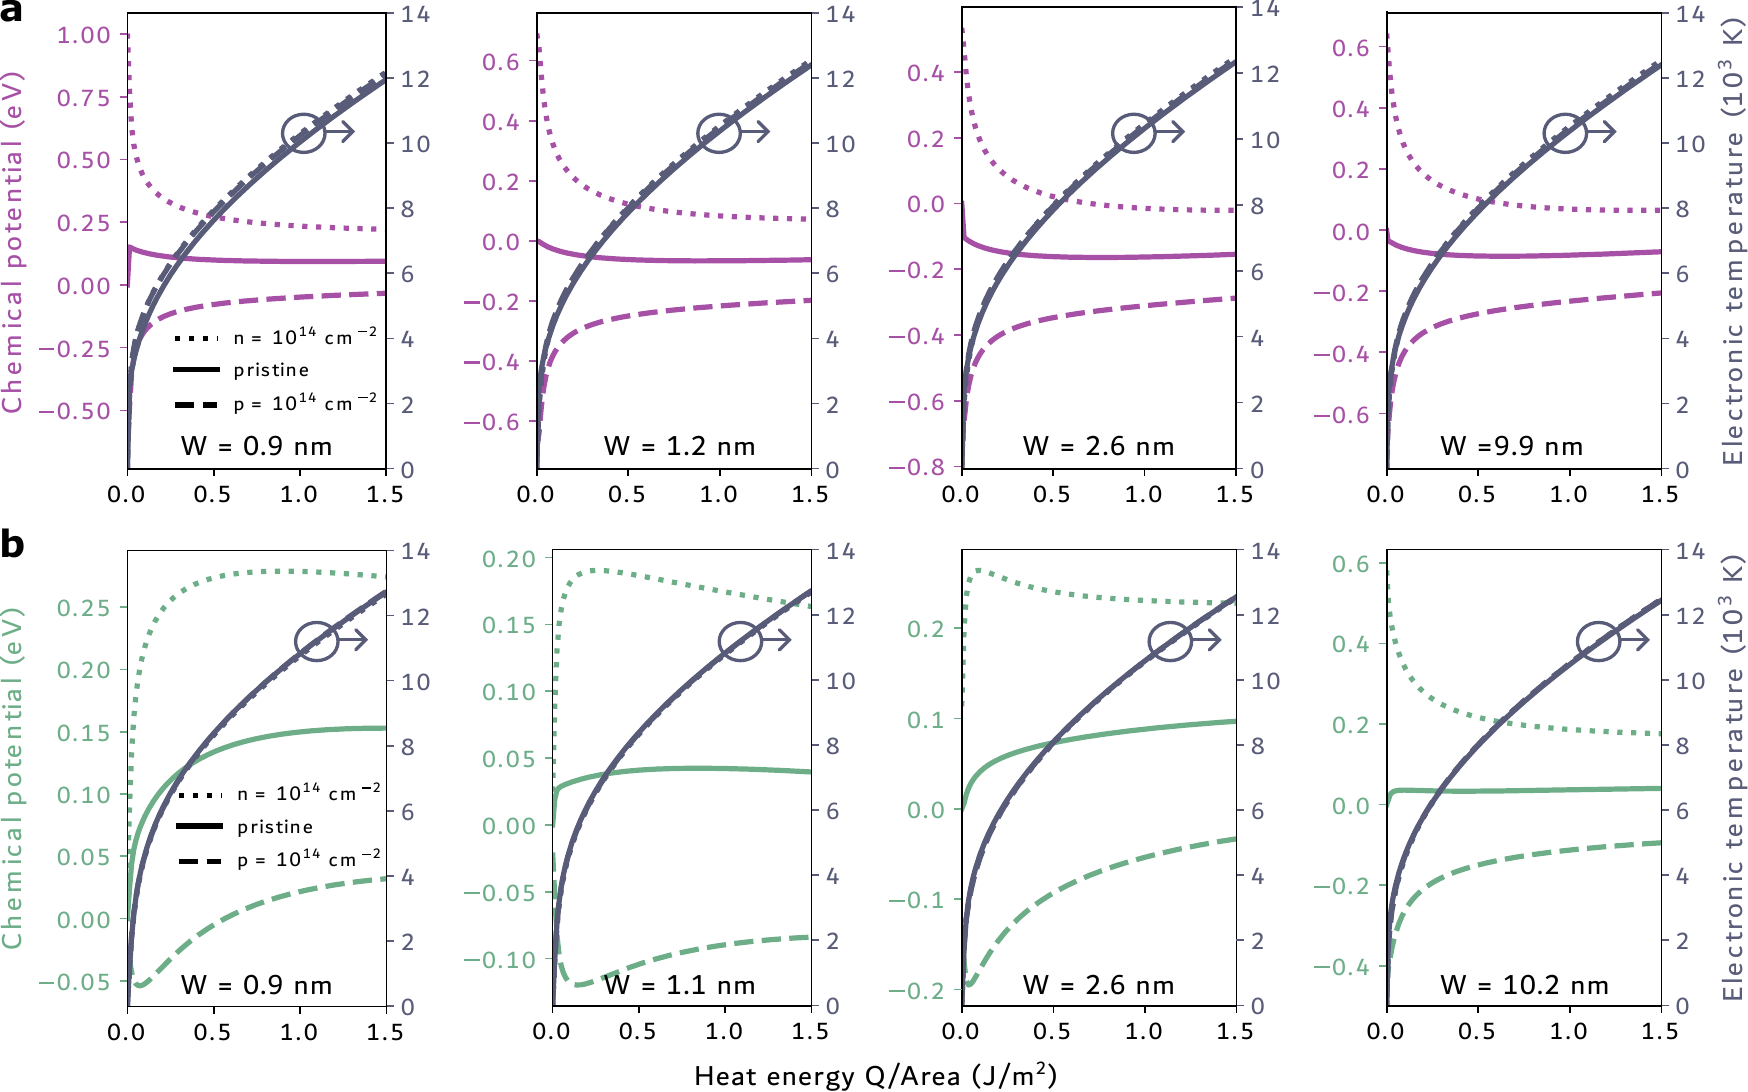}
    \caption{\textbf{Effect of heat energy density on the electronic distributions in graphene nanoribbons.} The electronic temperature and chemical potential determined from Eqs.~(2) and (3) in the main text are shown as functions of the added thermal energy $Q$ per unit area for the \textbf{a} AC and \textbf{b} ZZ GNRs of width $W$ considered in Fig.~\ref{fig:figS2} at high electron (dotted curves) and hole (dashed curves) doping densities, contrasted with undoped GNRs (solid curve).}
    \label{fig:figS4}
\end{figure*}

\begin{figure*}
    \centering
    \includegraphics[width=0.95\textwidth]{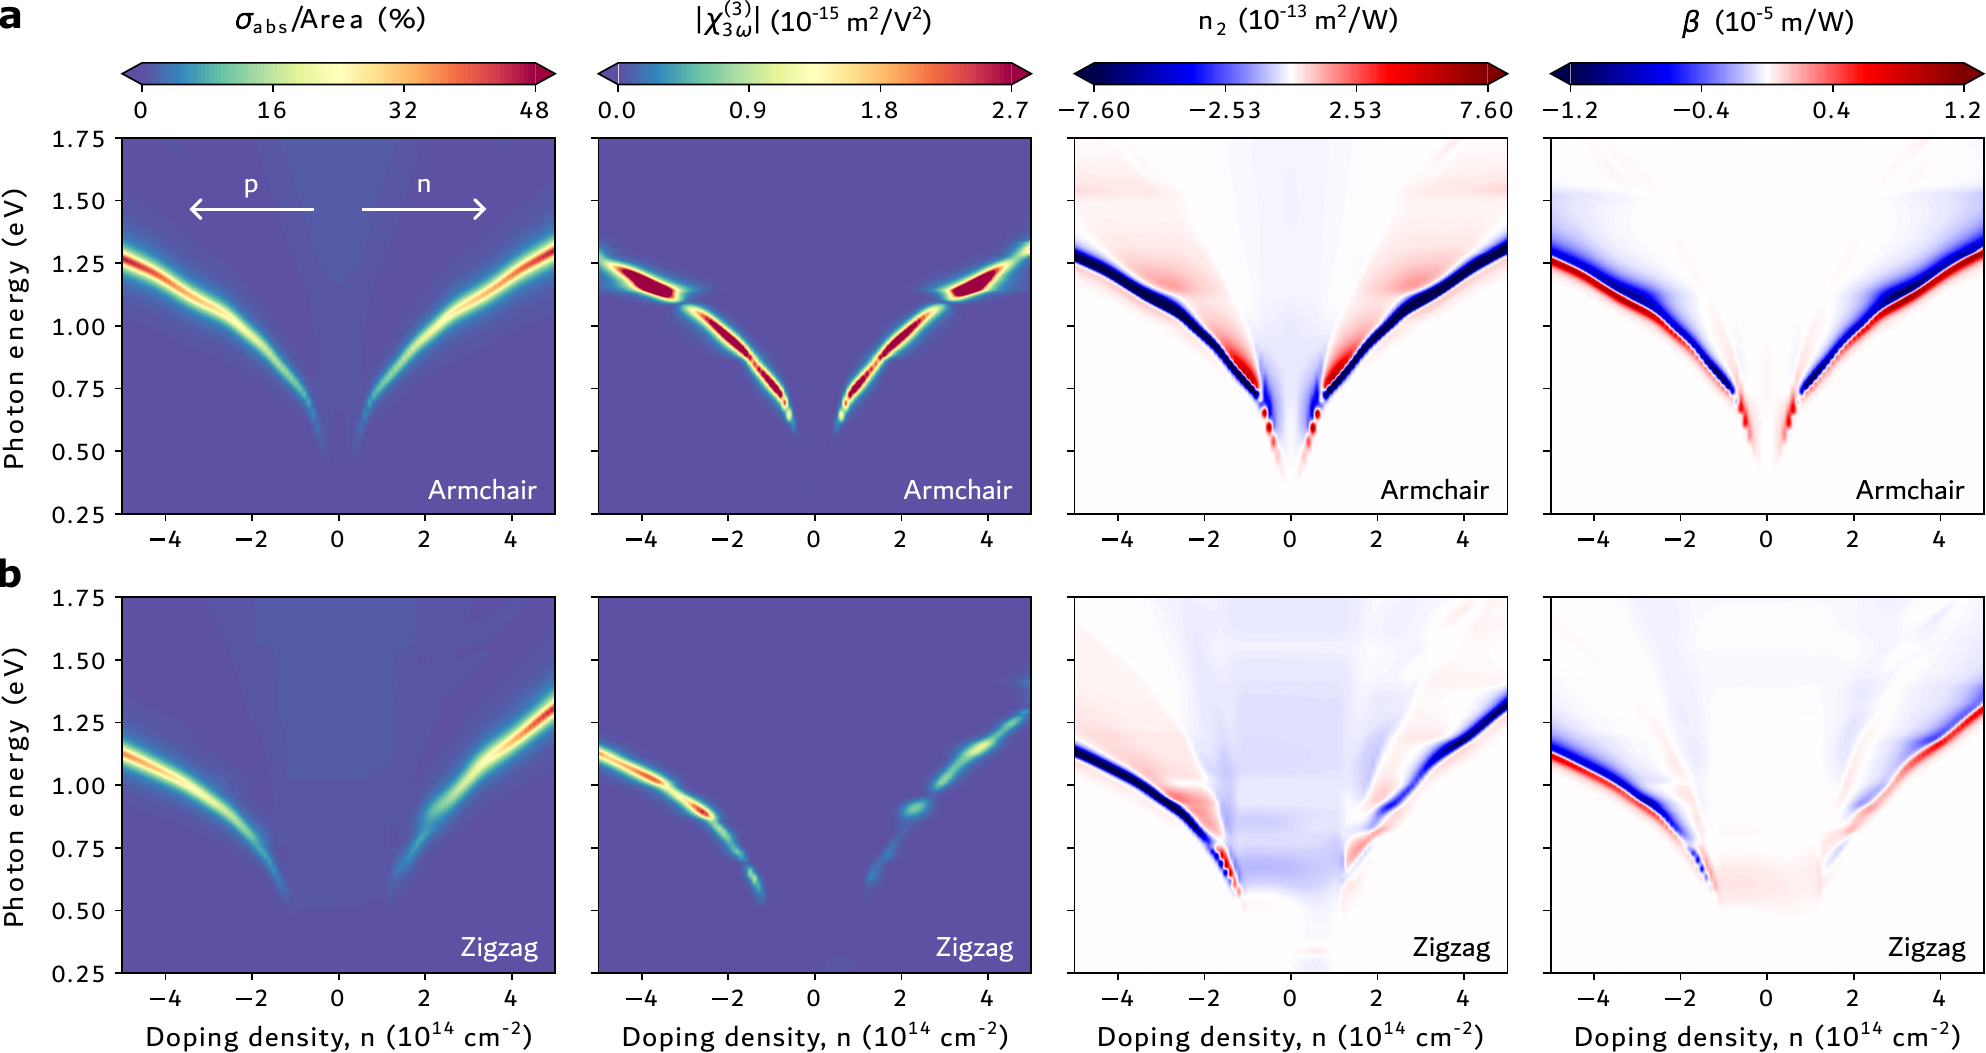}
    \caption{\textbf{Carrier density control of graphene plasmons.} The linear and nonlinear spectral response of \textbf{a} armchair and \textbf{b} zigzag edge-terminated GNRs with $W\approx 5$\,nm width at room temperature (300\,K) are shown over a continuous range of charge carrier doping levels spanning hole ($p$) and electron ($n$) doping.}
    \label{fig:figS3}
\end{figure*}

%\bibliographystyle{apsrev4-2}
%\bibliography{refs}

%apsrev4-2.bst 2019-01-14 (MD) hand-edited version of apsrev4-1.bst
%Control: key (0)
%Control: author (72) initials jnrlst
%Control: editor formatted (1) identically to author
%Control: production of article title (-1) disabled
%Control: page (0) single
%Control: year (1) truncated
%Control: production of eprint (0) enabled
%

\end{document}
